# Supplementary material for: Fixed Points and Noetherian Topologies
Source: arXiv:2207.07614 source file (2022-10-17)
Supplement: Supplementary file 1 [file appendix.tex]

\section{Quasi-orders}

\begin{definition}[Quasi-order]
    A binary relation $\leq$ over a set $X$
    is a quasi-order if it is reflexive and transitive.
\end{definition}

\begin{definition}[Good sequence]
    A sequence $(x_n)_{n \in \mathbb{N}} \in X^\mathbb{N}$
    of $(X, \leq)$ is a good sequence if $\exists i < j,
    x_i \leq x_j$.
    A sequence is bad when it is not a good sequence.
\end{definition}

\begin{definition}[Well-quasi-order]
    A quasi-ordered space $(X,\leq)$ is a well-quasi-order
    if all sequences are good sequences.
\end{definition}

\begin{definition}[Upwards closed sets]
    A set $A \subseteq X$ is upwards closed for $\leq$ in $X$
    when $\forall x \in A, \forall y \in X, x \leq y \implies y \in A$.
    Let us write ${\uparrow} A \defined \{ y \in X ~|~ \exists x \in A, x \leq y
    \}$ the upwards-closure of $A$ in $X$.
\end{definition}

\begin{definition}[Lattice]
    A lattice $L$ is a quasi-ordered space
    such that binary suprema and infima exists for all pairs of elements.
    A lattice is bounded when it has a top element and a bottom element.
    Equivalently, any finite infima and suprema exists in a bounded lattice.
\end{definition}

\begin{definition}[Boolean algebra]
\end{definition}

\begin{definition}[Boolean combination]

\end{definition}

\section{General Topology}

\begin{definition}[Topological space]
    A topological space is a pair $(X,\uptau)$
    where $\uptau$ is a collection of subsets of $X$
    stable under finite intersection and arbitrary union
    containing $\emptyset$ and $X$.
\end{definition}

\begin{definition}[Continuous map]
    A map $f : (X, \uptau) \to (Y, \uptheta)$ is continuous
    if $\forall U \in \uptheta, f^{-1}(U) \in \uptau$.
\end{definition}

\begin{definition}[Homeomorphism]
    A map $f : (X, \uptau) \to (Y, \uptheta)$ is a homeomorphism
    when $f$ is a bijection, $f$ is continuous, and $f^{-1}$ is
    continuous.
\end{definition}

\begin{definition}[Open cover]
    Let $(X,\uptau)$ be a topological space and $Y \subseteq X$,
    and open cover of $Y$ is a collection $(U_i)_{i \in I}$
    of open sets of $X$ such that $Y \subseteq \bigcup_{i \in I} U_i$.
    A cover is $\emph{finite}$ when $I$ is finite.
\end{definition}

\begin{definition}[Sub-cover]
    Let $(X,\uptau)$ be a topological space, $Y \subseteq X$
    and $(U_i)_{i \in I}$ be an open cover of $Y$,
    a sub-cover is a collection $(U_i)_{i \in I_0}$ where
    $I_0 \subseteq I$.
\end{definition}

\begin{definition}[Compactness]
    Let $(X,\uptau)$ be a topological space, a subset $Y \subseteq X$
    is compact if for any open cover of $Y$,
    one can extract a finite open sub-cover for $Y$.
\end{definition}

\begin{definition}[Induced topology]
    Consider a space $(X,\uptau)$ and a subset $Y \subseteq X$,
    the induced topology $\uptau_{|Y}$ is defined as
    $\uptau_{|Y} \defined \{ U \cap Y ~|~ U \in \uptau \}$.
\end{definition}

\begin{definition}[Basis]
    A base $\mathcal{B}$ of a topological space $(X,\uptau)$
    is a collection of open sets such that for all $U \in \uptau$,
    there exists $(B_i)_{i \in I} \in \mathcal{B}^I$ such that
    $U = \bigcup_{i \in I} B_i$.
\end{definition}

\begin{definition}[Sub base]
    A sub base $\mathcal{B}$ of a topological space $(X,\uptau)$
    is a collection of open sets such that $\mathcal{B}' \defined \left\{ \bigcap_{i
        \in I} B_i ~|~ I \text{ finite } \wedge (B_i)_{i \in I} \in
    \mathcal{B}^I \right\}$ is a base of $(X,\uptau)$.
\end{definition}

\begin{definition}[Generated topology]
    Let $X$ be a space and $\mathcal{B}$ be a collection of subsets of $X$,
    the topology $\generated{\mathcal{B}}$ generated by $\mathcal{B}$ is the smallest topology containing
    $\mathcal{B}$. Remark that $\mathcal{B}$ is then a sub base of the
    topology.
\end{definition}

\begin{definition}[Product topology]
    Consider spaces $(X_i, \uptau_i)_{i \in I}$
    the topological product is the space $X \defined \prod_{i \in I} X_i$
    with the topology generated by the \emph{cylinder open sets},
    that is, sets $\prod_{i \in I} U_i$ where $U_i \in \uptau_i$ 
    and $U_i \neq X_i$ for only finitely many indices.
\end{definition}

\begin{definition}[Image topology]
    Consider $(X,\uptau)$ a topological space
    and a function $f : X \to Y$.
    The image topology of $Y$ from $X$ through $f$
    is the smallest topology such that $f$ is continuous.
\end{definition}

\begin{definition}[Sum topology]
    Let $(X,\uptau)$ and $(Y,\uptheta)$ be two topological space,
    the sum space is $(X + Y, \uptau + \uptheta)$ where
    $\uptau + \uptheta$ is the topology generated by
    the union $\uptau \cup \uptheta$.
\end{definition}

\begin{definition}[Irreducible set]
    Let $(X,\uptau)$ be a non-empty topological space,
    it is reducible whenever there exists $U_1$ and $U_2$ two non-empty
    disjoint open sets such that $X = U_1 \cup U_2$.
    A subset $Y \subseteq X$ is reducible when it is reducible with the induced
    topology. An irreducible set is a set that is not reducible.
\end{definition}

\begin{definition}[Nœtherian space]
    A topological space $(X,\uptau)$ is Nœtherian
    if every subset $Y \subseteq X$ is compact.
\end{definition}

\begin{definition}[Alexandroff topology]
    A topology $\uptau$ over a space $X$ is an Alexandroff
    topology if $\uptau$ is stable under arbitrary intersection.
\end{definition}

\begin{definition}[Alexandroff topology of a quasi-order]
    Let $(X,\leq)$ a quasi-ordered space,
    the Alexandroff topology $\Alex{\leq}$ is the set
    of all $\leq$-upwards closed sets of $X$.
\end{definition}

\begin{lemma}[Compact in Alexandroff]
    Let $(X,\leq)$ be a quasi-ordered space,
    and $Y$ be an open set of $X$. The set $Y$ is a compact open set of $(X, \Alex{\leq})$
    if and only if $Y = {\uparrow}_\leq F$ where $F$ is a finite set of $X$.
\end{lemma}

\begin{definition}[Cofinite topology]
    Let $X$ be a set, let us write $\CofTop$ the collection of subsets of $X$
    sets whose complements are finite. This forms the \emph{cofinite} topology over $X$.
    Remark that this topology is always Nœtherian.
\end{definition}

\begin{definition}[Sober space]
    A space $(X,\uptau)$ is sober whenever
    every irreducible closed set is the
    closure of exactly one point.
\end{definition}

\begin{definition}[Sobrification]
\end{definition}

\begin{definition}[Spectral space]
    A topological space $(X,\uptau)$ is a spectral space
    if there exists a bases of compact open subsets of $X$
    stable under finite union and finite intersection such that
    $X$ is a sober space.
\end{definition}

\begin{definition}[Compact open subsets]
    Let $(X,\uptau)$ be a topological space,
    write $\CompSat{X}$ the set of compact open subsets of $X$.
\end{definition}

\begin{definition}[Spectral map]
    A function $f : X \to Y$ is a spectral map if it is continuous
    and $\forall U \in \CompSat{Y}, f^{-1}(U) \in \CompSat{X}$.
\end{definition}

\section{Logic}

\begin{definition}[Formula in $\FO$]
    Formulas in $\FO[\upsigma]$ are defined using the following 
    grammar

    \begin{align*}
        \phi \defined& R(x_1, \dots x_n) & R \in \upsigma \\
        |& \phi \wedge \phi ~|~ \phi \vee \phi \\
        |& \neg \phi ~|~ \exists x. \phi \\
        |& \forall x. \phi
    \end{align*}
\end{definition}

\begin{definition}[Free variable]
    Free variables of a formula are defined inductively
    \begin{align*}
        \FV(R(x_1, \dots, x_n)) &\defined \{ x_1, \dots, x_n \} \\
        \FV(\phi \wedge \psi) &\defined \FV(\phi) \cup \FV(\psi) \\
        \FV(\phi \vee \psi) &\defined \FV(\phi) \cup \FV(\psi) \\
        \FV(\neg \phi) &\defined \FV(\phi) \\
        \FV(\exists x. \phi) &\defined \FV(\phi) - \{ x \} \\
        \FV(\forall x. \phi) &\defined \FV(\phi) - \{ x \} 
    \end{align*}
\end{definition}

\begin{definition}[Sentence]
    A sentence is a formula $\phi$ having no free variable.
\end{definition}

\begin{definition}[Quantifier rank]
    The quantifier rank of a formula is defined inductively
    \begin{align*}
        \rk(R(x_1, \dots, x_n)) &\defined 0 \\
        \rk(\phi \wedge \psi) &\defined \max(\rk(\phi), \rk(\psi)) \\
        \rk(\phi \vee \psi) &\defined \max(\rk(\phi), \rk(\psi)) \\
        \rk(\neg \phi) &\defined \rk(\phi) \\
        \rk(\exists x. \phi) &\defined \rk(\phi) + 1 \\
        \rk(\forall x. \phi) &\defined \rk(\phi) + 1
    \end{align*}
\end{definition}

\begin{definition}[$\EFO$]
    A sentence $\phi \in \FO$ is an existential sentence
    if it is of the form $\exists x_1, \dots, x_n. \psi$
    where $\psi$ is quantifier free.
\end{definition}

\begin{definition}[$\EPFO$]
    A sentence $\phi \in \FO$ is an existential positive sentence
    if it is of the form $\exists x_1, \dots, x_n. \psi$
    where $\psi$ is quantifier free and contains no negation.
\end{definition}

\begin{definition}[$\PFO$]
    A sentence $\phi \in \FO$ is in $\PFO$ whenever
    it is of the form $\exists x_1, \dots, x_n. \psi$
    where $\psi$ is quantifier free, contains no negation
    except in front of the equality relation.
    In practice, this is a $\EPFO$ formula over the signature
    $\upsigma \uplus \{ \neq \}$.
\end{definition}

\begin{definition}[Ehrenfeucht-Fraïse game]
\end{definition}

\begin{definition}[Gaifman Distance]
    Let $A \in \Mod(\upsigma)$, $a \in A$ and $b \in A$,
    the distance $\dist(a,b)$ is the length of the shortest
    path from $a$ to $b$ in $\Gaif{A}$.
\end{definition}

\begin{fact}
    For all $r \in \mathbb{N}$, for all $\upsigma$ \emph{finite}
    relational signature
    there exists a formula $\dist(x,y) \leq r$
    such that
    for all $A \in \Mod(\upsigma)$,
    $A, ab \models \dist(x,y)\leq r$ if and only if
    $a \in \Neighb{A}{b}{r}$ or equivalently 
    if and only if $b \in \Neighb{A}{a}{r}$.
\end{fact}

\begin{definition}[Local neighborhood]
    Let $A \in \Mod(\upsigma)$
    $a \in A$, $r \in \mathbb{N}$,
    $\Neighb{A}{a}{r} \defined \{ b \in A ~|~ \dist(a,b) \leq r \}$.
    The neighborhood of a tuple $\vec{a}$
    is the unions of the neighborhoods of each element.
\end{definition}

\begin{definition}[Relativized formulas]
    The relativisation of a formula
    $\phi$ with free variables $\vec{x}$
    to $\Neighb{}{\vec{x}}{r}$
    is obtained inductively as follows
    \newcommand{\Relativise}[3]{\mathcal{R}_{#1}^{#2}\left(#3\right)}
    \begin{align*}
        \Relativise{r}{\vec{x}}{R(y_1, \dots y_n)} &\defined R(y_1, \dots, y_n)
        \\
        \Relativise{r}{\vec{x}}{\phi \wedge \psi} &\defined
        \Relativise{r}{\vec{x}}{\phi} \wedge
        \Relativise{r}{\vec{x}}{\psi} \\
        \Relativise{r}{\vec{x}}{\phi \vee \psi} &\defined
        \Relativise{r}{\vec{x}}{\phi} \vee
        \Relativise{r}{\vec{x}}{\psi} \\
        \Relativise{r}{\vec{x}}{\neg \phi} &\defined
        \neg \Relativise{r}{\vec{x}}{\phi} \\
        \Relativise{r}{\vec{x}}{\exists y. \phi} &\defined
        \exists y. y \in \Neighb{}{\vec{x}}{r} \wedge 
        \Relativise{r}{\vec{x}}{\phi} \\
    \end{align*}
    Where
    \begin{equation*}
    y \in \Neighb{}{\vec{x}}{r}
    \defined
    \bigvee_{x_i \in \vec{x}}
    \dist(y,x_i) \leq r
    \end{equation*}
\end{definition}

\begin{definition}[Local sentences and formulas]
    A formula $\phi$ with $n$ free variables $\vec{x}$
    is $r$-local if 
    $\forall A, \forall \vec{a} \in A^n,
        A, \vec{a} \models \phi
        \iff
        \Neighb{A}{\vec{a}}{r}, \vec{a} \models \phi$.
\end{definition}

\begin{definition}[Basic local sentence]
    A sentence $\phi$ is a basic local sentence of radius $r$
    if it is written
    $\exists \vec{x}. \psi$ where $\psi$ is relativized to
    $\Neighb{}{\vec{x}}{r}$.
\end{definition}

\begin{theorem}[Gaifman locality theorem]
    Any formula $\phi \in \FO$ is a boolean combination of local formulas and
    basic local sentences.
\end{theorem}

\begin{definition}[Local type]
    Given a structure $A \in \Mod(\upsigma)$,
    a tuple $\vec{a} \in A^n$, a radius $r$ and a quantifier bound $n$,
    the local type of $\vec{a}$,
    $\NeighbT{A}{\vec{a}}{r}{n}$, the set of all formulas
    of quantifier rank less than $n$ with $|\vec{a}|$ variables
    that are true in $\Neighb{A}{\vec{a}}{r}$.
    Note that there are only finitely many possible local types
    given $r,n$.
\end{definition}

\section{Graphs and structures}

\begin{definition}[Structure]
    Let $\upsigma$ be a relational signature,
    an element $A \in \Mod(\upsigma)$ is
    a domain $|A|$ and relations of the form $\Rel{R}{A}{x_1, \dots, x_n}$
    in $|A|^n$ for each symbol $R \in \upsigma$ of arity $n$.
    A structure is finite if $|A|$ is a finite set.
\end{definition}

\begin{definition}[Homomorphism]
    Let $A$ and $B$ be two elements of $\Mod(\upsigma)$,
    a homomorphism $f : A \to B$ is a function $f : |A| \to |B|$
    such that
    \begin{equation*}
        \forall R \in \upsigma,
        \forall (x_1, \dots, x_n) \in |A|^n,
        \Rel{R}{A}{x_1, \dots, x_n} \implies \Rel{R}{B}{f(x_1), \dots, f(x_n)}
    \end{equation*}
\end{definition}

\begin{definition}[Strong Homomorphism]
    Let $A$ and $B$ be two elements of $\Mod(\upsigma)$,
    a strong homomorphism $f : A \to B$ is a function $f : |A| \to |B|$
    such that
    \begin{equation*}
        \forall R \in \upsigma,
        \forall (x_1, \dots, x_n) \in |A|^n,
        \Rel{R}{A}{x_1, \dots, x_n} \iff \Rel{R}{B}{f(x_1), \dots, f(x_n)}
    \end{equation*}
\end{definition}

\begin{definition}[Substructure]
    Let $A$ and $B$ be two elements of $\Mod(\upsigma)$,
    $A$ is a substructure of $B$ if there exists an injective homomorphism from
    $A$ to $B$.
\end{definition}

\begin{definition}[Induced substructure]
    Let $A$ and $B$ be two elements of $\Mod(\upsigma)$,
    $A$ is a substructure of $B$ if there exists a strong homomorphism from $A$
    to $B$.
\end{definition}

\begin{definition}[Graph]
    A graph is an element $A$ of $\Mod(\{ (E,2) \})$
    such that there is no element $u \in |A|$
    such that $\Rel{E}{A}{u,u}$.
\end{definition}

\begin{definition}[Gaifman graph]
    Let $A \in \Mod(\upsigma)$,
    the Gaifman graph $\Gaif{A}$ is
    the graph with domain $|A|$ 
    and $\Rel{E}{A}{u,v}$ if and only if
    there exists a relation $R \in \upsigma$
    such that $u$ and $v$ appear in a tuple of the relation.
\end{definition}

\begin{definition}[Tree-depth~\protect{\cite[Definition 6.1]{Neetil12}}]
    The tree-depth of a graph $G$ is the minimum height of a
    forest $F$ with the property that every edge of $G$ connects a pair of nodes
    that have an ancestor-descendant relationship to each other in $F$.

    Equivalently, the tree depth is characterized by the following recursive
    definition
    \begin{equation*}
        td(G)=\begin{cases}1, & \text{if }|G|=1;\\
        1+\min_{v\in V} td(G-v), & \text{if }G\text{ is connected and }|G|>1;\\
        \max_{i} td(G_i), &\text{otherwise};
        \end{cases}
    \end{equation*}
\end{definition}

\begin{definition}[Clique-width]
\end{definition}

\begin{definition}[Hereditary, monotone class]
\end{definition}

\begin{definition}[Wideness]
\end{definition}

\begin{definition}[Nowhere dense]
\end{definition}

\subsection{Topologically Indecomposable Words}

In the study of the \kl{regular subword topology},
words $w$ satisfying that every cut $w = uv$
with $v \neq \varepsilon$
$\adh{w} = \adh{v}$ are of particular interest.
Those words are called \intro{topologically indecomposable}
and are the ``word'' counterpart to indecomposable ordinals.
These are particularly useful as every word $w$
is a finite product of such \kl{topologically indecomposable words}.

\begin{lemma}[Decomposition]
	\label{lem:tf:irreddecomp}
	Every word $w$ is a product
	of finitely many \kl{topologically
		indecomposable words}.
\end{lemma}
\begin{proof}
	By induction on the ordinal size of the word $|w|$
	and its closure $\adh{w}$ which is well-founded
	because the \kl{recurrent subword topology}
	is \kl{Noetherian}.

	If $w$ is \kl{topologically indecomposable},
	we have written $w$ as a finite product of \kl{topologically
		indecomposable} words.

	Otherwise, there exists $u,v$ such that
	$w = uv$, $v \neq \varepsilon$, and $\adh{v} \subsetneq \adh{w}$.
	Notice that $|u| < |w|$, $|v| \leq |w|$, $\adh{u} \subseteq \adh{w}$,
	and $\adh{v} \subseteq \adh{w}$.
	We can therefore apply our induction hypothesis on $u$ and $v$
	to conclude that they both are expressible as
	a finite product of \kl{topologically
		indecomposable words}, hence that $w$ is too.
\end{proof}

\begin{lemma}
	If $v \in \adh{u}$ then $|v| \leq |u|$.
\end{lemma}
\begin{proof}
	This is a direct consequence of $u \in \adh{u} \subseteq X^{<|u|+1}$.
\end{proof}

\begin{lemma}[Size of a \kl{topologically indecomposable} word]
	A \kl{topologically indecomposable} word has an
	indecomposable size.
\end{lemma}
\begin{proof}
	Let us write $w$ of size $\beta = \gamma + \delta$
	as a product $uv$ with $|u| = \gamma$ and $|v| = \delta$.
	Because $w \in \adh{v}$, $|w| \leq |v|$ hence $\delta = \beta$.
\end{proof}

\begin{lemma}[Closure of a product]
	\label{lem:ft:closureproduct}
	Let $w_1, \dots, w_n$ be \kl{topologically indecomposable} words.
	Then $\adh{w_1 \dots w_n} = \adh{w_1} \dots \adh{w_n}$.
\end{lemma}
\begin{proof}
	We consider separately the different ways to obtain an irreducible
	closed set.
	\begin{enumerate}
		\item If it is obtained as $C^{\leq 1}$ with $C$ closed in $\theta$.
		      There can be at most one letter in $w$,
		      hence the equality holds trivially because $n = 1$.
		\item If it is obtained as $P^{<\beta}$ with $P$ closed.
		      Then $w \in P^{<|w|+1}$, hence $\beta = |w|+1$.
		      In particular, this proves that $P^{<\beta} = P^{<|w_1|+1} \dots
			      P^{<|w_n|+1}$.
		      Assume by contradiction that $\adh{w_i} \subsetneq P$.
		      Then, $w_1 \dots w_n \in P_1^{<|w_1|+1} \dots \adh{w_i}^{<|w_i|+1}
			      \dots P_n^{|w_n|+1}$
		      which contradicts the minimality of $P^{<\beta}$.
		\item If it is obtained as $P_1 \dots P_m$ for some $m \in \mathbb{N}$.
		      Then $w = u_1 \dots u_m$ with $u_i \in P_i$.
		      Let us denote $f(j)$ the index $i$ such that $u_i$
		      contains a suffix of $w_j$.
		      Because $w_j$ is indecomposable,
		      $\adh{w_j} \subseteq \adh{u_{f(j)}} \subseteq P_{f(j)}$.
		      In particular, $\adh{w_1} \dots \adh{w_n} \subseteq
			      P_1 \dots P_m = \adh{w_1 \dots w_n}$.
		      Conversely, $\adh{w_1 \dots w_n}$ is always contained
		      in $\adh{w_1} \dots \adh{w_n}$ as the latter is a
		      closed subset containing $w_1 \dots w_n$.
	\end{enumerate}
\end{proof}

\begin{corollary}
	\label{cor:ft:closureproduct}
	The closure $\adh{w_1 \dots w_n}$
	equals $\adh{w_1} \dots \adh{w_n}$ in general.
\end{corollary}
\begin{proof}
	Decompose each $w_i$ into finitely
	many \kl{topologically indecomposable words}
	using \cref{lem:tf:irreddecomp}
	and conclude using \cref{lem:ft:closureproduct}.
\end{proof}

As a consequence, computing the specialisation
preorder amounts to computing the
closure of \kl{topologically indecomposable words}.

\subsection{Approximating Closed Sets}

In the \kl{recurrent subword topology},
there are some basic closed sets that
are the topological counterpart to
\kl{topologically indecomposable words}.
Precisely, we call a closed set $C$ \intro{atomic}
whenever $C \subseteq C_1 \cdot C_2$ implies
$C \subseteq C_1$ or $C \subseteq C_2$.
It is immediate that $\adh{w}$
is \kl{atomic} whenever $w$ is \kl{topologically
	indecomposable},
but there are more examples.
For instance $X^*$ is \kl{atomic} and
cannot be obtained as the closure of a word.

The goal of this section is to provide
ways to approximate \kl{irreducible}
and \kl{atomic} closed sets using unions of
closures of
words.

\kvdef{ApxFam}{\mathcal{F}}
\begin{definition}[Approximant]
	A family $\intro*\ApxFam_C$ of words in $X^{<\alpha}$
	\intro{approximates}
	a set $C$ whenever
	$C = \adh{\ApxFam_C} = \bigcup_{w \in \ApxFam_C} \adh{w}$.

	An \intro{approximant} of a set $C$ is a
	family $\ApxFam_C$ that \kl{approximates} $C$,
	is directed for $\HigLeq$,
	downwards closed, and satisfies
	that for every split $w = w_A w_B$
	of words in the family,
	either $\setof{w_A}{w \in \ApxFam_C}$
	or $\setof{w_B}{w \in \ApxFam_C}$ \kl{approximates} $C$.
\end{definition}

Given a topologically indecomposable word $w$,
it is clear that ${\downarrow} w$ is an \kl{approximant}
for $\adh{w}$. Indeed, it is a downwards closed, directed
set of words, and splitting $w = w_A w_B$ either
produces $w_B \neq \varepsilon$, in which case $\adh{w_B} = \adh{w}$
or $w_B = \varepsilon$ in which case $w = w_A$.
Notice that whenever
$\ApxFam_C$ is an \kl{approximant} of $C$,
one can consider $C$ itself as an approximant.
Moreover, approximable closed sets are
automatically \kl{irreducible} and \kl{atomic}.

\begin{lemma}[Approximable sets are atomic]
	Let $\ApxFam_C$ be an \kl{approximant} for a closed set $C$,
	and $A,B$ be closed sets.
	If $C \subseteq A \cdot B$,
	either $C \subseteq A$ or $C \subseteq B$.
\end{lemma}
\begin{proof}
	For every $w \in \ApxFam_C$, we have
	$w \in A \cdot B$, hence $w = w_A w_B$
	for some $w_A \in A$ and $w_B \in B$.
	Because $\ApxFam_C$ is an \kl{approximant},
	either
	$C = \bigcup_{w \in \ApxFam_C} \adh{w_A} \subseteq A$
	or
	$C = \bigcup_{w \in \ApxFam_C} \adh{w_B} \subseteq B$.
\end{proof}

\begin{lemma}[Approximable sets are irreducible]
	Let $\ApxFam_C$ be an \kl{approximant} for a closed set $C$,
	and $A,B$ be closed sets.
	If $C \subseteq A \cup B$,
	either $C \subseteq A$ or $C \subseteq B$.
\end{lemma}
\begin{proof}
	For every $w \in \ApxFam_C$, we have
	$w \in A \cup B$, hence $w = w_A w_B$
	for some $w_A \in A$ and $w_B \in B$.
	Concretely, we let $w_A = w$ and $w_B = \varepsilon$
	if $w \in A$ (resp. $w_A = \varepsilon$, $w_B = w$
	if $w \in B$).
	Because $\ApxFam_C$ is an \kl{approximant},
	either
	$C = \bigcup_{w \in \ApxFam_C} \adh{w_A} \subseteq A$
	or
	$C = \bigcup_{w \in \ApxFam_C} \adh{w_B} \subseteq B$.
\end{proof}

Let us briefly check that $X^*$ it is an \kl{approximant} of $X^*$:
it is downwards closed and directed.
Let us select at splitting $w = w_A w_B$ for every finite word,
and prove that either $\bigcup_{w \in X^*} \adh{w_A} = X^*$
or $\bigcup_{w \in X^*} \adh{w_B} = X^*$.
Assume by contradiction that both equality fails,
this provides a finite word $u_A$ that is not in
$\bigcup_{w \in X^*} \adh{w_A}$
and a finite word $u_B$ that is not in
$\bigcup_{w \in X^*} \adh{w_B}$.
Consider now $w = u_A u_B$, it is a finite word, hence is split
in $w_A w_B$, but whatever the split, either $u_A \in \adh{w_A}$
or $u_B \in \adh{w_B}$, which is absurd.

Remark that being approximable is \emph{a priori} a stronger
property than being \kl{irreducible} and \kl{atomic}.
Indeed, the latter properties are splitting the sets or
cutting the words \emph{with respect to some closed sets}
whereas we allow arbitrary cuts in an \kl{approximant}.
We will however prove that whenever $X$ is a \kl{sober} space,
\kl{atomic} and \kl{irreducible} closed set are
approximable.

\begin{lemma}
	\label{lem:tf:irredclosedsets}
	Assume that $X$ is \kl{sober}.
	Irreducible closed subsets of the
	\kl{recurrent subword topology}
	are obtained through the derivations
	depicted in \cref{fig:trans:closed-sets},
	and are directed with respect to $\HigLeq$.
\end{lemma}
\begin{proof}
	Let us say that $C$ is derivable whenever it can be
	obtained by the rules in \cref{fig:trans:closed-sets}.
	A finite intersection of derivable sets
	can be rewritten as
	a finite union of derivable sets. Since
	the \kl{recurrent subword topology} is \kl{Noetherian}
	and derivable sets generate the topology,
	every closed set is a finite intersection of finite unions
	of derivable sets, hence a finite union of derivable sets.

	We prove the affirmation that \kl{irreducible}
	closed sets are directed by induction on the derivation.
	It is trivial for $C^{\leq 1}$ because it is the
	closure of a single point, and holds by induction
	hypothesis for the products
	and iterations.
\end{proof}

\begin{lemma}[Atomic irreducible closed sets are approximable]
	\label{lem:tf:atomicirredappx}
	Assume that $X$ is \kl{sober}.
	Let $C$ be an irreducible atomic closed set.
	There exists an \kl{approximant} $\ApxFam_C$ of $C$.
\end{lemma}
\begin{proof}
	We prove the result by a case analysis
	on the shape of
	of the irreducible closed set via the rules of
	\cref{fig:trans:closed-sets} thanks to
	\cref{lem:tf:irredclosedsets}.

	\begin{description}
		\item[Case $C^{\leq 1}$]
		      Because $C^{\leq 1}$ is \kl{irreducible},
		      $C$ must be \kl{irreducible} in $X$.
		      As $X$ is \kl{sober}, this proves that
		      there exists a letter $x \in X$
		      such that $C = \adh{x}^X$.
		      We define $\ApxFam_{C^{\leq 1}}$
		      as ${\downarrow} x$.

		\item[Case $P_1 \dots P_n$]
		      Because the set is supposed \kl{atomic}
		      this reduces to the other cases.

		\item[Case $P^{\leq 1}$]
		      then $P^{\leq 1} = P$, and
		      this reduces to the other cases.

		\item[Case $P^{< \beta}$ with $\beta$ indecomposable]
		      Let us define $\ApxFam$ as $P^{<\beta}$ itself.
		      Let $w = w_A w_B$ be a split of the
		      words in $\ApxFam$.
		      Assume by contradiction that
		      $\bigcup_{w \in \ApxFam} \adh{w_A} \subsetneq P^{<\beta}$,
		      and
		      $\bigcup_{w \in \ApxFam} \adh{w_B} \subsetneq P^{<\beta}$.
		      This provides two words $w_1$ and $w_2$
		      that are in $P^{<\beta}$ but
		      not in $\bigcup_{w \in \ApxFam} \adh{w_A}$ (resp. $w_B$).

		      Because $\beta$ is indecomposable, $|w_1 w_2| < \beta$,
		      and $w_1 w_2 \in P^{<\beta}$.
		      As a consequence, it is split in two, but whatever the split,
		      this is in contradiction with our assumption on $w_1$ and $w_2$.

		\item[Case $P^{< \beta+1}$ with $\beta$ indecomposable]
		      Let us define $\ApxFam$ as $P^{<\beta+1}$ itself.
		      Let $w = w_A w_B$ be a split of the
		      words in $\ApxFam$.
		      Assume by contradiction that
		      $\bigcup_{w \in \ApxFam} \adh{w_A} \subsetneq P^{<\beta}$,
		      and
		      $\bigcup_{w \in \ApxFam} \adh{w_B} \subsetneq P^{<\beta}$.
		      This provides two words $w_1$ and $w_2$
		      that are in $P^{<\beta}$ but
		      not in $\bigcup_{w \in \ApxFam} \adh{w_A}$ (resp. $w_B$).

		      Thanks to \cref{lem:tf:irredclosedsets}, there exists
		      a word $w_3$ that is above $w_1$ and $w_2$ while
		      remaining in $P^{<\beta + 1}$.
		      Without loss of generality, assume that $|w_3| = \beta$,
		      which can be obtained by padding.
		      We will now rely on dark ordinal magic, namely
		      the \emph{Hessenberg pairing},
		      to build a word $w_4$, still in $P^{<\beta + 1}$, such that
		      every non-empty suffix of $w_4$ contains $w_3$,
		      which is absurd
		      with respect to the definition of $w_1$ and $w_2$.

		      Since $\beta$ is indecomposable, there exists
		      a function $H \colon \beta \times \beta \to \beta$
		      which is injective and satisfies that for all
		      $\delta_1 < \delta_2 < \beta$,
		      and $\delta_3 < \beta$,
		      $H(\delta_1, \delta_3) < H(\delta_2, \delta_3)$
		      and
		      $H(\delta_3, \delta_1) < H(\delta_3, \delta_2)$.
		      Because $w_3 \in P^{<\beta + 1}$,
		      there exists a map
		      $f \colon \beta \to P$
		      such that $w_3 = \prod_{\gamma < \beta} f(\gamma)$.
		      Let us define
		      $g(H(\delta_1, \delta_2)) \defined f(\delta_2)$
		      for $\delta_1, \delta_2 < \beta$,
		      and $g(\delta) = 0$ if $\delta$ is not in the range
		      of $H$.
		      This allows us to write the word
		      $w_4 \defined \prod_{\gamma < \beta} g(\gamma)$.

		      Let us now split $w_4$ at a position $\gamma < \beta$,
		      since $H(\gamma, 0) \geq \gamma$,
		      we find $w_3$ as a subword in the suffix.
		      \qedhere
	\end{description}
\end{proof}

\subsection{Computing the Stature}

\begin{lemma}
	Assume that $X$ is \kl{sober}.
	Let $A,B$ be two closed sets,
	and let $P_1, \dots, P_n$ be non-empty \kl{irreducible}
	\kl{atomic} closed sets.
	If $P_1 \dots P_n \subseteq AB$
	there exists $1 \leq i \leq n$
	such that $P_1 \dots P_i \subseteq A$,
	and $P_{i+1} \dots P_n \subseteq B$.
\end{lemma}
\begin{proof}
	Thanks to \cref{lem:tf:atomicirredappx},
	$P_1, \dots, P_n$ are \kl{approximated}
	by families $P_1, \dots, P_n$.

	Let us say that a word
	$w = w_1 \cdots w_n$ \emph{splits at position} $i$
	whenever the part of $w = w_A w_B$
	is such that $w_B$ contains a non-empty suffix of
	$w_i$. By convention, let us say that
	$w$ \emph{splits at position} $n+1$
	whenever $w_B = \varepsilon$. Hence, every word $w = w_1 \cdots w_n$
	splits at a position
	between $1$ and $n+1$.

	Let $m$ be the maximal index
	between $1$ and $n+1$ such that
	for every $w$ in $P_1 \cdots P_n$
	there exists a $w'$
	\emph{pointwise above} $w$ for $\HigLeq$
	such that $w'$ splits at position $m$.

	Notice that this index must exist,
	otherwise for every $1 \leq i \leq n+1$
	there exists a word $u_i$ such that
	for every $u_i \HigLeq w'$
	$w'$ cannot split at position $i$.
	Because $P_1, \dots, P_n$ are directed,
	one can build an element $u$ above
	$u_i$ for $1 \leq i \leq n$.
	This element cannot split at any index,
	which is absurd, since $u \in A B$.

	Because $P_m$ is \kl{approximated} by itself, either
	$P_m$ equals $\bigcup_{w_m \in P_m} \adh{w_m^A}$
	or $P_m$ equals $\bigcup_{w_m \in P_m} \adh{w_m^B}$.
	Assume without loss of generality
	that $P_m = \bigcup_{w_m \in P_m} \adh{w_m^A}$.
	We will prove that
	$P_1 \dots P_m \subseteq A$ and
	$P_{m+1} \dots P_n \subseteq B$.

	Consider a word $w' = w_1' \dots w_n'$
	in $P_1 \dots P_n$.
	It is pointwise below some word $w$
	that splits as position $m$.
	Hence, $\adh{w_i'} \subseteq \adh{w_i}$,
	$\adh{w_1} \dots \adh{w_{m-1}} \adh{w_m^A} \subseteq A$,
	and
	$\adh{w_{m+1}} \dots \adh{w_n} \subseteq B$.
	In particular,
	$P_1 \dots P_m \subseteq A$,
	and $P_{m+1} \dots P_n \subseteq B$.
\end{proof}

\begin{lemma}
	Assume that $X$ is \kl{sober},
	let $P,Q$ be closed sets
	and $\beta,\gamma$ be ordinals of the form
	$\beta'$ or $\beta'+1$ with $\beta'$ indecomposable.
	If $P^{<\beta} \subseteq Q^{<\gamma}$
	then $P \subseteq Q$ and
	$\beta \leq \gamma$.
\end{lemma}
\begin{proof}
	This is completely false
\end{proof}

\begin{definition}
	Let us define $|P^{< \beta}| = |P|^{\beta}$,
	$|P_1 \dots P_n| = \oplus_{i = 1}^n |P_i|$
	and $|C^{\leq 1}|$ as the rank of $C$ in $X$.
\end{definition}

\begin{theorem}
	The stature of the \kl{recurrent subword topology}
	is bounded by $\varepsilon_0$... cool
\end{theorem}
